# Supplementary material for: Introducing "Forecast Utterance" for Conversational Data Science
Source: arXiv:2309.03877 source file (2023-09-07)
Supplement: Supplementary file 1 [file online_resources.tex]

\section*{Online Resources}

\begin{urlist}
\item\label{OpenRefine}\url{http://openrefine.org/}
\item\label{TrifactaWrangler}\url{https://www.trifacta.com/products/wrangler/}
\item\label{Drake}\url{https://github.com/Factual/drake}
\item\label{TIBCOClarity}\url{https://clarity.cloud.tibco.com/landing/feature-summary.html}
\item\label{DataQuality}\url{https://sourceforge.net/projects/dataquality/})
\item\label{Winpure}\url{https://winpure.com/}
\item\label{TalentedDataQuality}\url{https://www.trustradius.com/products/talend-data-quality/reviews}
\item\label{DataLadder}\url{https://dataladder.com/}
\item\label{DataCleaner}\url{https://datacleaner.org/}
\item\label{Cloudingo}\url{https://cloudingo.com/}
\item\label{Refier}\url{http://nubetech.co/technology/}
\item\label{IBMInfosphereQualityStage}\url{https://www.ibm.com/uk-en/marketplace/infosphere-qualitystage}
\item\label{FeatureTools}\url{https://www.featuretools.com/}
\item\label{featexp}\url{https://github.com/abhayspawar/featexp}
\item\label{MLFeatureSelection}\url{https://github.com/duxuhao/Feature-Selection}
\item\label{FeatureEngineeringFeatureSelection}\url{https://github.com/Yimeng-Zhang/feature-engineering-and-feature-selection}
\item\label{FeatureHub}\url{https://github.com/HDI-Project/FeatureHub}
\item\label{featuretoolsR}\url{https://github.com/magnusfurugard/featuretoolsR}
\item\label{Feast}\url{https://cloud.google.com/blog/products/ai-machine-learning/introducing-feast-an-open-source-feature-store-for-machine-learning}
\item\label{ExploreKit}\url{https://github.com/giladkatz/ExploreKit}
\item\label{HyperparameterHunter}\url{https://github.com/HunterMcGushion/hyperparameter_hunter}
\item\label{AmazonSagemaker}\url{https://aws.amazon.com/sagemaker/}
\item\label{hyperband}\url{https://github.com/zygmuntz/hyperband}
\item\label{BigMLOptiML}\url{https://bigml.com/api/optimls}
\item\label{Hyperboard}\url{https://github.com/WarBean/hyperboard}
\item\label{GoogleHyperTune}\url{https://cloud.google.com/ml-engine/docs/using-hyperparameter-tuning}
\item\label{SHERPA}\url{https://github.com/sherpa-ai/sherpa}
\item\label{IndieSolver}\url{https://indiesolver.com/}
\item\label{Milano}\url{https://github.com/NVIDIA/Milano}
\item\label{MindFoundryOPTaaS}\url{https://www.mindfoundry.ai/mind-foundry-optimize}
\item\label{BBopt}\url{https://github.com/evhub/bbopt}
\item\label{sigopt}\url{https://sigopt.com/}
\item\label{adatune}\url{https://github.com/awslabs/adatune}
\item\label{gentun}\url{https://github.com/gmontamat/gentun}
\item\label{optuna}\url{https://github.com/optuna/optuna}
\item\label{test-tube}\url{https://github.com/williamFalcon/test-tube}
\item\label{Advisor}\url{https://github.com/tobegit3hub/advisor}
\item\label{DotData}\url{https://dotdata.com/}
\item\label{TPOT}\url{https://github.com/EpistasisLab/tpot}
\item\label{IBMAutoAI}\url{www.ibm.com/Watson-Studio/AutoAI}
\item\label{Auto-Sklearn}\url{https://github.com/automl/auto-sklearn}
\item\label{AzureMachineLearning}\url{https://azure.microsoft.com/en-us/services/machine-learning/}
\item\label{GoogleCouldAIplatform}\url{https://cloud.google.com/ai-platform/}
\item\label{AmazoonAWSservice}\url{https://aws.amazon.com/marketplace/solutions/machine-learning/data-science-tools}
\item\label{DataRobot}\url{https://www.datarobot.com/}
\item\label{AmazonForecast}\url{https://aws.amazon.com/forecast/}
\item\label{AutoKeras}\url{https://github.com/keras-team/autokeras}
\item\label{H2ODriverlessAI}\url{http://docs.h2o.ai/driverless-ai/latest-stable/docs/userguide/index.html}
\item\label{AdaNet}\url{https://github.com/tensorflow/adanet}
\item\label{CloudAutoML}\url{https://cloud.google.com/automl/}
\item\label{PocketFlow}\url{https://github.com/Tencent/PocketFlow}
\item\label{C3AISuite}\url{www.c3.ai}
\item\label{automl-gs}\url{https://github.com/minimaxir/automl-gs}
\item\label{FireFly}\url{www.firefly.ai}
\item\label{MLBox}\url{https://github.com/AxeldeRomblay/MLBox}
\item\label{Builton}\url{www.builton.dev/ml-apis}
\item\label{Morph-net}\url{https://github.com/google-research/morph-net}
\item\label{DeterminedAIPlatform}\url{www.determined.ai}
\item\label{ATM}\url{https://github.com/HDI-Project/ATM}
\item\label{TransmogrifAI}\url{https://github.com/salesforce/TransmogrifAI}
\item\label{RemixAutoML}\url{https://github.com/AdrianAntico/RemixAutoML}
\item\label{OpenML100}\url{https://www.openml.org/s/14}
\item\label{OpenML-CC18}\url{https://www.openml.org/s/98}
\item\label{AutoMLChallenges}\url{http://automl.chalearn.org/data}
\end{urlist}
